# Supplementary material for: RibSeg v2: A Large-scale Benchmark for Rib Labeling and Anatomical Centerline Extraction
Source: arXiv:2210.09309 source file (2023-08-01)
Supplement: Supplementary file 1 [file supp.tex]

\section{Supplementary Material}
\subsection{Ablation Study on Rib Segmentation}
\label{subsec:exp_seg}

\subsubsection{Evaluation Metrics}
To evaluate the performance of rib labeling, we report the segmentation Dice\cite{Dice1945MeasuresOT, Taha2015MetricsFE}, defined as
\begin{equation}
Dice^{(S)}=\sum_i |y_i\cdot \hat{y}_i|/(|y|+|\hat{y}|),
\end{equation} 

where $y$ and $\hat{y}$ indicate the predicted label and ground truth, respectively. Apart from segmentation performance, we also report the missing ratio of individual ribs to evaluate the clinical applicability of the method. Specifically, a missing of an individual rib $i$ is counted if $\textit{recall}_i<0.5$, and then the missing ratio can be calculated with ease. Considering that segmenting first and twelfth rib pairs tend to be more difficult as they are shorter and more curvy than other ribs, we calculate and report the missing ratio of all / first / intermediate / twelfth rib pairs respectively, as depicted in Tab.~\ref{tab:seg_metrics1}. 

\subsubsection{Quantitative Analysis}
For method comparison, we first implement a voxel-based 3D-UNet~\cite{cciccek20163d} taking patches of CT volumes as input with the same setting of FracNet~\cite{jin2020deep}. Moreover, we tested the point-based PointNet++ with different settings, including Absolute-and-Relative-Positioning, Points-Augmentation and Connected-Components-Denoising. 

\textbf{Metrics analysis}.
As depicted in the Tab.~\ref{tab:seg_metrics1}, point-based methods significantly outperform voxel-based 3D-UNet. For missing rib ratio, the point-based method performs well on the overall pairs of ribs, while suffering drops on the floating ribs. An interpretation is that the various lesion on floating ribs makes it hard to segment. For example, in some cases, the floating ribs are extremely short or vague, and in a small amount of cases, the floating ribs are missing or there is a third stubby little floating rib, which are difficult to segment. Besides, for method comparison, by enriching the local geometric representation, the ARP mechanism improves the performance on Segmentation Dice by $1.73\%$, and rib missing ratio by $0.77\%/2.72\%/0.33\%/3.56\%$, on average. The performance improvement of applying PA is relatively slight on this task, with $1.58\%$ on Segmentation Dice and $0.56\%/1.42\%/0.17\%/4.10\%$ on rib missing ratio. While CCD has a numerically small boost of $1.53\%$ on Segmentation Dice, and $0.49\%/0.95\%/0.28\%/2.58\%$ on rib missing ratio, we showed that it is crucial to rib labeling and centerline extraction as reported in Tab.~\ref{tab:label_metrics} and Tab.~\ref{tab:cl_metrics}. Overall, the method performs best on rib segmentation task is point-based method with ARP, PA, and CCD.

\subsubsection{Qualitative Analysis}
Results with a high Dice value may not necessarily have a visually satisfying segmentation, as the data distributions of different ribs are quite different from each other, especially for the floating ribs. Hence, we report several visualization results from the test set, and conduct quality analysis to explore general problems in rib segmentation.

\textbf{General analysis}.
For most cases, the predicted segmentations are promising, it's even hard to tell the difference between predictions and ground truths, just like the cases in Fig.~\ref{fig:seg_vis_good}~(a). While in some cases, the prediction contains a few mis-segmented voxels, which can be easily fixed through morphological post-processing. For example, the prediction in Fig.~\ref{fig:seg_vis_good}~(b) contains a small part of the scapula that can be nicely filtered by post-processing. To make the experiment practically critical, we also report the result of some abnormal yet clinically common cases, which are also surprisingly nice. For instance, even for cases with serious scoliosis, like Fig.~\ref{fig:seg_vis_good}~(c), where the spine is horribly twisted, the predicted segmentation is still almost flawless. And for cases with incomplete rib cage, as depicted in the Fig.~\ref{fig:seg_vis_good}~(d), the prediction is also visually qualified for clinical applications.

\textbf{Performance degradation analysis}. 
The model suffers performance degradation in a few cases, where some major misclassifications occur. Hence, we analyze those cases and summarize them to the following conditions:
\begin{enumerate}
    \item   cases that contain noise due to the deviations in the HU values
    \item   cases that contain irregular objects with dense voxels
    \item   cases where the floating ribs are too short or contain too sparse voxels
\end{enumerate}

\begin{figure}[tph]
    \centering
	\includegraphics[width=\linewidth]{fig/seg_vis_good.png}
	\caption{\textbf{Visualization of Segmentation Predictions}. (a) The case is normal, and its prediction is flawless. (b) The case is normal, but its prediction contains part of the scapula and a few noises. (c) The case contains serious scoliosis. (d) The case contains an incomplete rib cage.} \label{fig:seg_vis_good}
\end{figure}

\begin{figure}[tph]
    \centering
	\includegraphics[width=\linewidth]{fig/seg_vis_bad.png}
	\caption{\textbf{Visualization of Performance Degradation}. (a) The case suffers HU deviation, and the prediction contains too many noises. (b) The case contains an inseparable pacemaker, and the prediction contains a large part of the pacemaker. (c) The case contains the floating ribs that are short and vague, and the prediction of floating ribs is sparse.} \label{fig:seg_vis_bad}
\end{figure}

As depicted in Fig.~\ref{fig:seg_vis_bad}~(a), in the input binary volume, the rib cage is wrapped by a 'noise shell', which causes many noise points left in the prediction. Such 'noise shell' is caused by the deviation in HU value, i.e., the HU value of the voxels is higher/lower than their normal HU value. For a normal case, thresholding by a HU value of 200 can filter most non-bone regions and leave a clean rib cage, however, for some cases suffering a deviation in HU value, the resultant binary volume will contain numerous noises. In \emph{RibSeg v2} dataset, there exists 3 causes for HU deviation:
\begin{enumerate}
    \item   Some cases contain metal implants, a deviation of HU value will be caused when X-ray passing through the implants, and artifacts may be generated as well.
    \item   For some cases, the patient might be overweight and have rather large body shape, which will affect the attenuation of X-ray, causing the HU deviation. Normally, the tube voltage (kV) and milliampere-seconds (mAs) of the X-ray should be adjusted according to the body size of patients, however, there might be artificial or systematic errors leading to an insufficient X-ray intensity, which also increases the noise in the region of interest. 
    \item   A few cases contain the volumes of arm bones, which will also cause the HU deviation. Such case could occur when the patient is not able to raise his/her arms in the scanning process due to some injury.
\end{enumerate}

To tackle such problems, we apply CCD to the binarized CT scans to eliminate the noise. Specially, for the binarized CT scans, we sort the connected components by their volume and take the largest 100 components, which is a safe number to keep all rib voxels while filtering the majority of noises. Note that in the cases containing comminuted fracture, the connected components of ribs could be unexpectedly large. The prediction on the denoised data has much less noise and a tremendously improved Dice performance, as reported in the Fig.~\ref{fig:denoise} and Tab.~\ref{tab:seg_metrics1}. And the next subsection also shows that CCD is crucial to generating accurate label predictions.

As depicted in Fig.~\ref{fig:seg_vis_bad}~(b), the case contains a pacemaker outside the patient's body, whose high density could disturb the data distribution. Although the prediction contains the majority of the rib voxels, there are still visually obvious voxels of pacemakers remained. This actually urges a potential improvement that to make the model more geometrically robust by applying a rib template as prior constraints. 

As depicted in Fig.~\ref{fig:seg_vis_bad}~(c) where the floating ribs are shorter than normal cases and contain very sparse voxels, and in the prediction, the predicted floating ribs are even more sparse. Such case is not rare in clinical, and the challenges could be twofold: sparsity and less neighboring correlation. a) It is clinically common that the floating ribs tend to be shorter and more curvy, and the various lesion on floating ribs make them contain even less voxels. b) The floating ribs have less neighboring bones, which limits the feature extracted from adjacent ribs. Although the same problem exists for the top pair of the ribs, in our dataset, the top pairs of ribs contain sufficient voxels to alleviate the prediction error. However, it is still a potential challenge that the top pairs of ribs will have more distractions from neighboring bones, such as clavicles and scapula.

\begin{figure*}[tb]
    \centering
	\includegraphics[width=\linewidth]{fig/denoise_v2.png}
	\caption{\textbf{Comparison of Inferences with/without CCD (Connected Components Denoise)}. This figure shows the effects of applying CCD to the CT volumes, it includes the binarized volume, segmentation prediction, and label prediction. With CCD applied to the binarized CT volumes, the majority of noise points are eliminated from the binarized volume, and the method generates a more clean segmentation prediction, also improving the quality of label prediction. For the label prediction on the input applied by CCD, there exists little mislabeling, which can be easily eliminated by post-process. Colors in CT volumes and rib segmentation denote the axial depth, and the label palette indicates the label color assigned to each rib.} \label{fig:denoise}
\end{figure*}

\textbf{Dataset analysis}. During the experiment, we also notice that some predictions may contain a few rib voxels that are not included in the ground truth due to the ambiguity of annotation, i.e., the determination of the rib voxels and costal cartilage voxels are vague. Specifically, during the annotation, our priority is to make sure the intermediate main parts of the rib are included, while some parts of the bones connected to the spine or the costal cartilages could be cut off. Although such small neglection would not affect the overall segmentation quality, it remains a potential quality improvement for the \emph{RibSeg v2} dataset.
